# Supplementary material for: JOG3R: Towards 3D-Consistent Video Generators
Source: arXiv:2501.01409 source file (2025-03-26)
Supplement: Supplementary file 2 [file old_main_supp.tex]

% CVPR 2025 Paper Template; see https://github.com/cvpr-org/author-kit

\documentclass[10pt,twocolumn,letterpaper]{article}

%%%%%%%%% PAPER TYPE  - PLEASE UPDATE FOR FINAL VERSION
% \usepackage{cvpr}              % To produce the CAMERA-READY version
\usepackage[review]{cvpr}      % To produce the REVIEW version
% \usepackage[pagenumbers]{cvpr} % To force page numbers, e.g. for an arXiv version

% Import additional packages in the preamble file, before hyperref
\input{preamble}

% It is strongly recommended to use hyperref, especially for the review version.
% hyperref with option pagebackref eases the reviewers' job.
% Please disable hyperref *only* if you encounter grave issues, 
% e.g. with the file validation for the camera-ready version.
%
% If you comment hyperref and then uncomment it, you should delete *.aux before re-running LaTeX.
% (Or just hit 'q' on the first LaTeX run, let it finish, and you should be clear).
\definecolor{cvprblue}{rgb}{0.21,0.49,0.74}
\usepackage[pagebackref,breaklinks,colorlinks,allcolors=cvprblue]{hyperref}

%%%%%%%%% PAPER ID  - PLEASE UPDATE
\def\paperID{8303} % *** Enter the Paper ID here
\def\confName{CVPR}
\def\confYear{2025}

%%%%%%%%% TITLE - PLEASE UPDATE
%\title{Camera Pose Estimation Emerging in Video Diffusion Transformer}

\title{Supplementary Material:\\On Unifying Video Generation and Camera Pose Estimation}

%%%%%%%%% AUTHORS - PLEASE UPDATE
\author{First Author\\
Institution1\\
Institution1 address\\
{\tt\small firstauthor@i1.org}
% For a paper whose authors are all at the same institution,
% omit the following lines up until the closing ``}''.
% Additional authors and addresses can be added with ``\and'',
% just like the second author.
% To save space, use either the email address or home page, not both
\and
Second Author\\
Institution2\\
First line of institution2 address\\
{\tt\small secondauthor@i2.org}
}
\input{macro}
\begin{document}
\maketitle
\input{sec/10_suppmat}
% {
%     \small
%     \bibliographystyle{ieeenat_fullname}
%     \bibliography{iclr2025_conference}
% }

% WARNING: do not forget to delete the supplementary pages from your submission 
% \input{sec/X_suppl}

\end{document}
